# Supplementary material for: Smooth Convex Optimization using Sub-Zeroth-Order Oracles
Source: arXiv:2103.00667 source file (2021-03-01)
Supplement: Supplementary file 1 [file supp.tex]

\relax
%File: formatting-instructions-latex-2021.tex
%release 2021.1
\documentclass[letterpaper]{article} % DO NOT CHANGE THIS
\usepackage{aaai21}  % DO NOT CHANGE THIS
\usepackage{times}  % DO NOT CHANGE THIS
\usepackage{helvet} % DO NOT CHANGE THIS
\usepackage{courier}  % DO NOT CHANGE THIS
\usepackage[hyphens]{url}  % DO NOT CHANGE THIS
\usepackage{graphicx} % DO NOT CHANGE THIS
\urlstyle{rm} % DO NOT CHANGE THIS
  % DO NOT CHANGE THIS
\usepackage{natbib}  % DO NOT CHANGE THIS AND DO NOT ADD ANY OPTIONS TO IT
\usepackage{caption} % DO NOT CHANGE THIS AND DO NOT ADD ANY OPTIONS TO IT
\frenchspacing  % DO NOT CHANGE THIS
\setlength{\pdfpagewidth}{8.5in}  % DO NOT CHANGE THIS
\setlength{\pdfpageheight}{11in}  % DO NOT CHANGE THIS

\input{commands}
\usepackage{amsmath}

\usepackage[switch]{lineno}

\usepackage{amssymb}
\usepackage{dsfont}
\usepackage{enumerate}

\usepackage{amsthm}
\usepackage{graphicx}
\usepackage{algorithm}% http://ctan.org/pkg/algorithms
\usepackage{algpseudocode}% http://ctan.org/pkg/algorithmicx
\usepackage{tikz}
\usepackage{booktabs}
\usepackage{bbold}
\usetikzlibrary{automata, positioning, arrows}
\usepackage[utf8]{inputenc}
\usepackage[english]{babel}
\usepackage{mathtools}

\theoremstyle{definition}

\theoremstyle{definition}

\usepackage{wrapfig}

%\tikzset{
%	->, % makes the edges directed
%	>=stealth', % makes the arrow heads bold
%	initial text=$ $, % sets the text that appears on the start arrow
%}

\definecolor{purple}{rgb}{1,0.5,1}
\definecolor{green}{rgb}{0.5,1,0.5}
\definecolor{red}{rgb}{1,0.5,0.5}
\usepackage{xcolor}
\usepackage{subcaption}

\graphicspath{{images/}}

\algtext*{EndWhile}
\algtext*{EndFor}
\algtext*{EndFunction}
\algtext*{EndIf}

\tikzset{
	->, % makes the edges directed
	>=stealth', % makes the arrow heads bold
	initial text=$ $, % sets the text that appears on the start arrow
}

%\nocopyright
%PDF Info Is REQUIRED.
% For /Author, add all authors within the parentheses, separated by commas. No accents or commands.
% For /Title, add Title in Mixed Case. No accents or commands. Retain the parentheses.
\pdfinfo{
	/Title ()
	/Author ()
} %Leave this

\setcounter{secnumdepth}{0} %May be changed to 1 or 2 if section numbers are desired.

% The file aaai21.sty is the style file for AAAI Press
% proceedings, working notes, and technical reports.
%

% Title

% Your title must be in mixed case, not sentence case.
% That means all verbs (including short verbs like be, is, using,and go),
% nouns, adverbs, adjectives should be capitalized, including both words in hyphenated terms, while
% articles, conjunctions, and prepositions are lower case unless they
% directly follow a colon or long dash

\title{Supplementary Material for ``Smooth Convex Optimization using Sub-Zeroth-Order Oracles''}
\author{Author names are omitted for submission}

\definecolor{darkcandyapplered}{rgb}{0.64, 0.0, 0.0}
\definecolor{darkolivegreen}{rgb}{0.33, 0.42, 0.18}
\usepackage{tikz}

\begin{center}
	{ \huge \textbf{Supplementary Material for ``Smooth Convex Optimization using Sub-Zeroth-Order Oracles''}}
\end{center}
%\doublespacing

 	\linenumbers

We give the proofs for the technical results in this document. We also include the preliminaries for self-containment.

\input{prelims.tex}
\input{proofs.tex}

\clearpage
\bibliographystyle{aaai}
\bibliography{ref2}
